# Supplementary material for: Measuring the Prevalence of WiFi Bottlenecks in Home Access Networks
Source: arXiv:2311.05499 source file (2023-11-29)
Supplement: Supplementary file 1 [file appendix.tex]

\appendix
\section{Appendix}
